# Supplementary material for: EvaGaussians: Event Stream Assisted Gaussian Splatting from Blurry Images
Source: arXiv:2405.20224 source file (2024-12-06)

**Rendered  
Mode**

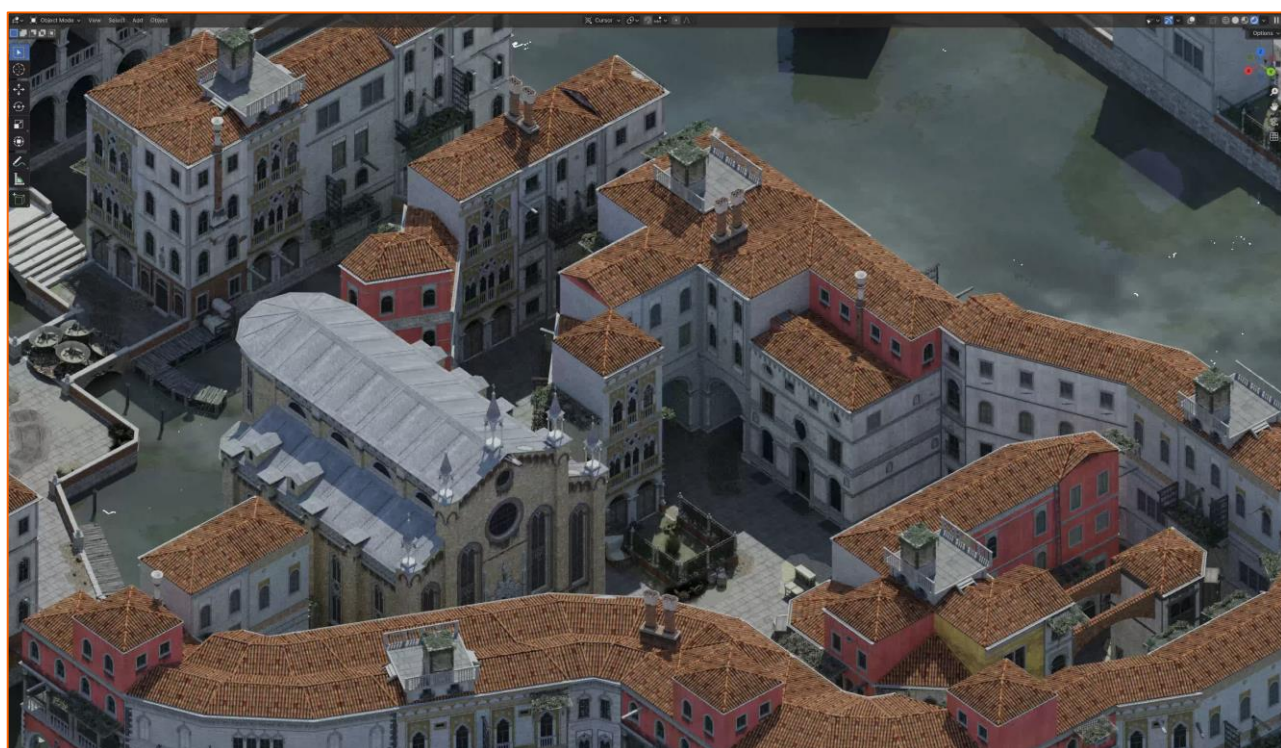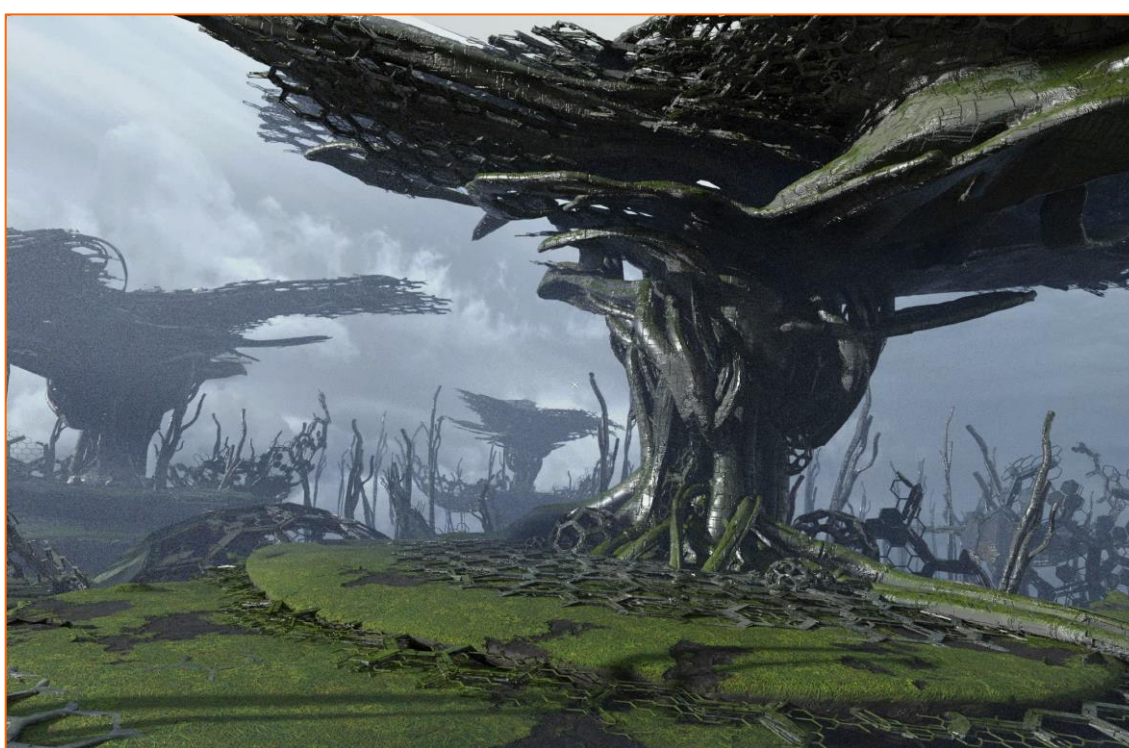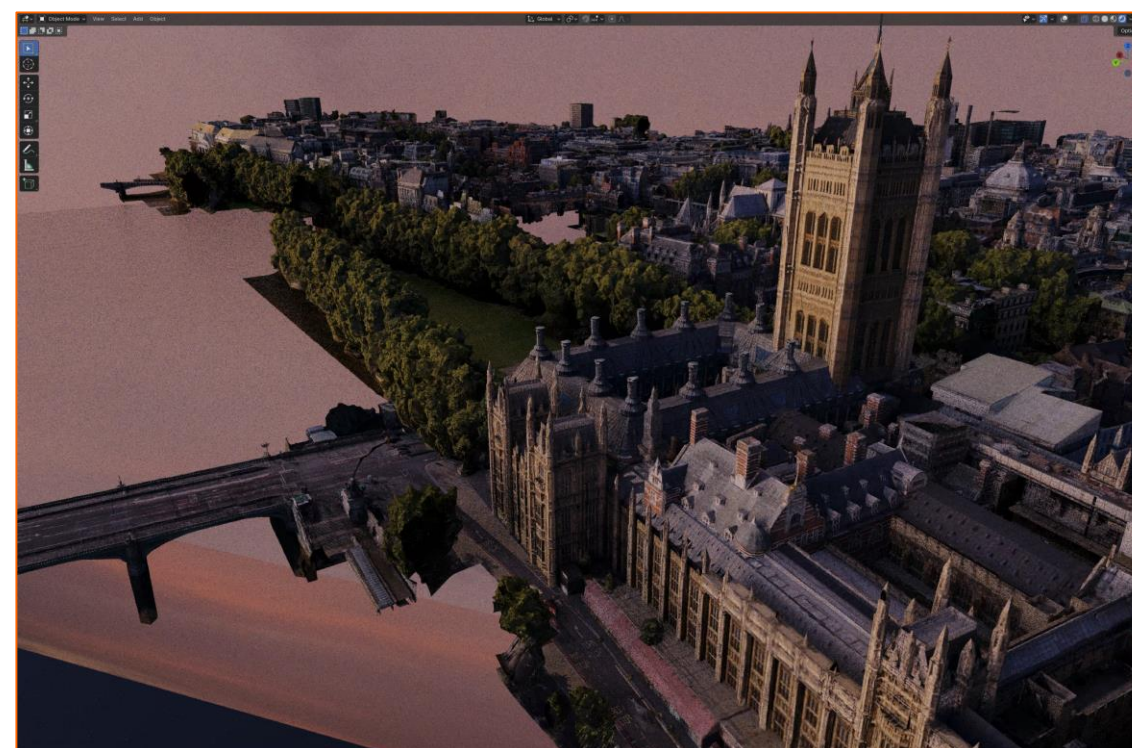

**WireFrame  
Mode**

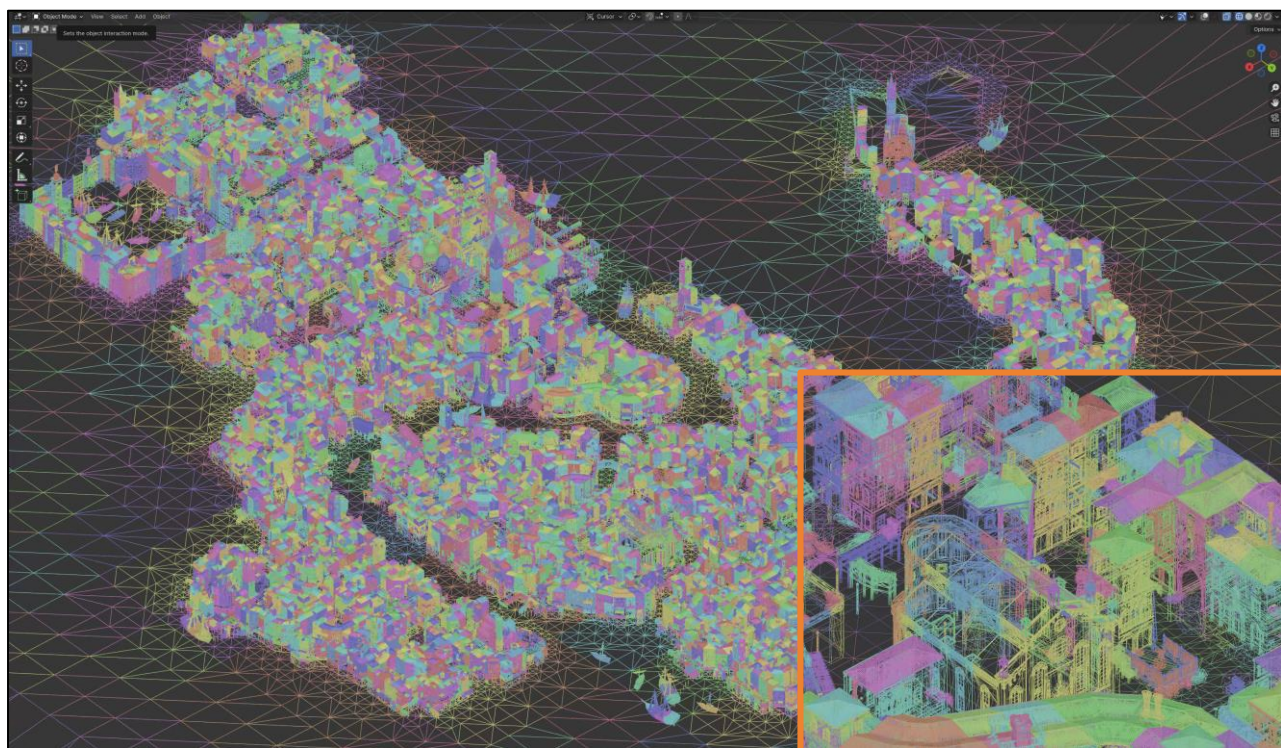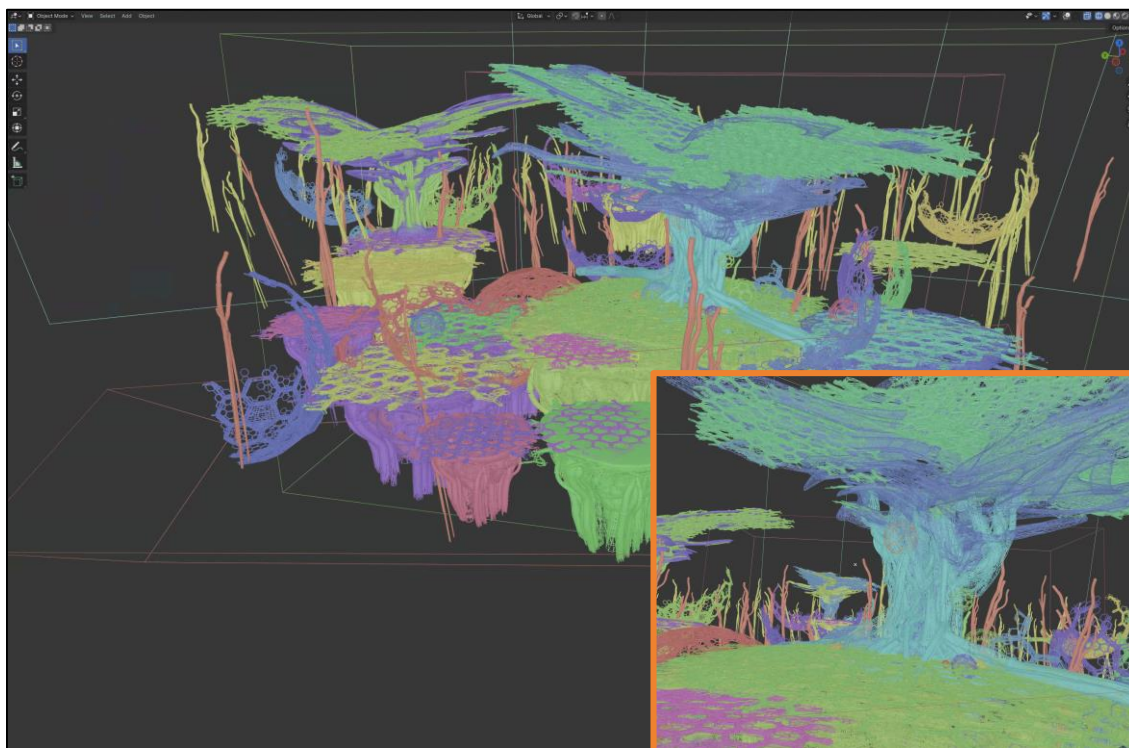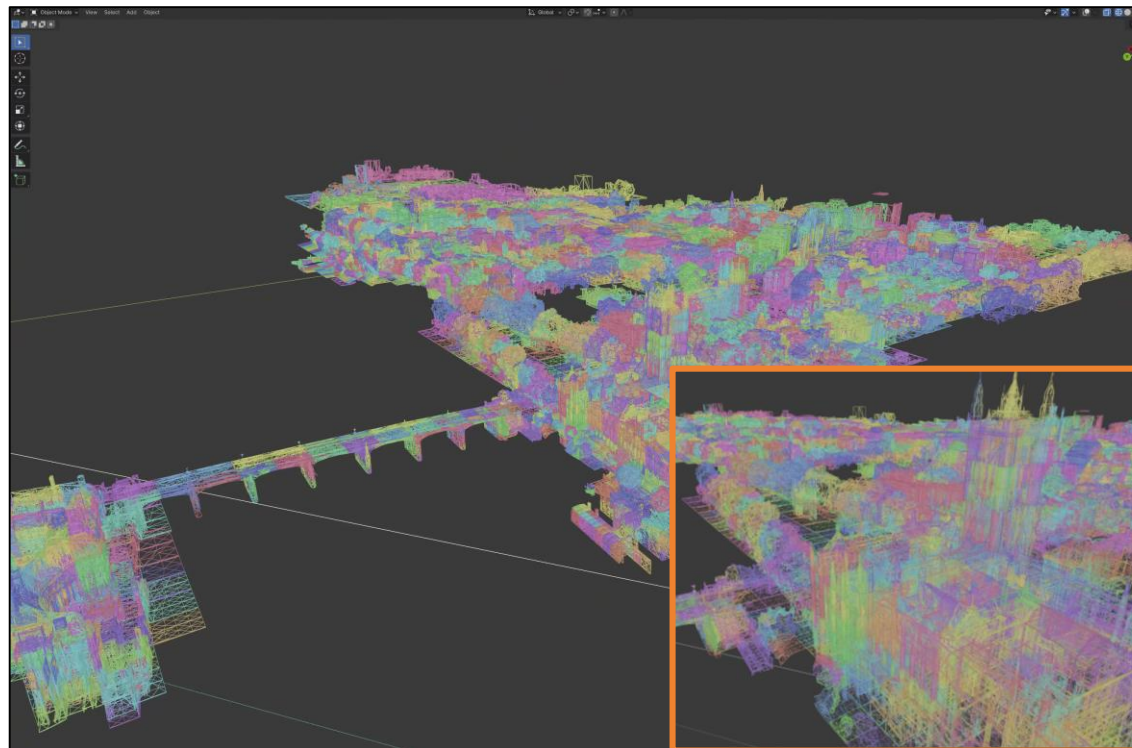

**Venice**

**Forests**

**London**

**Rendered  
Mode**

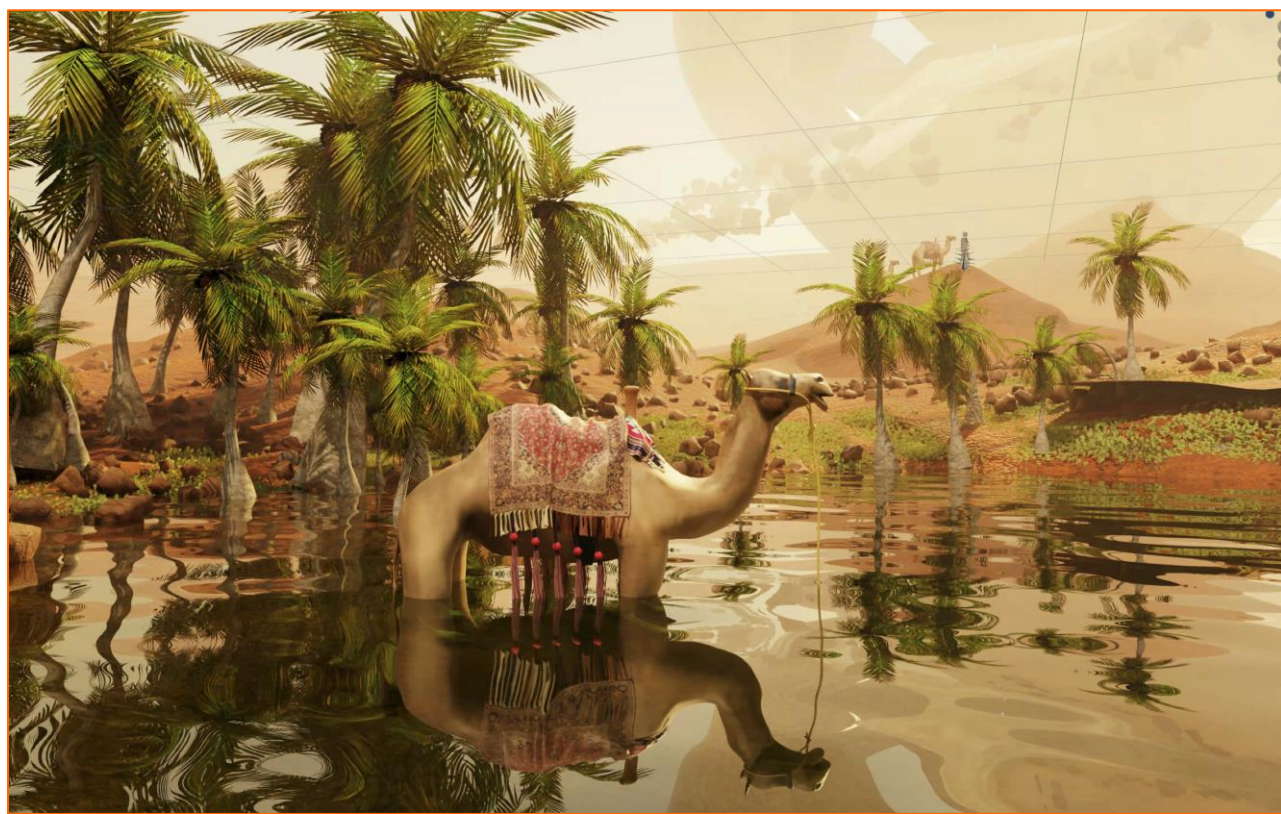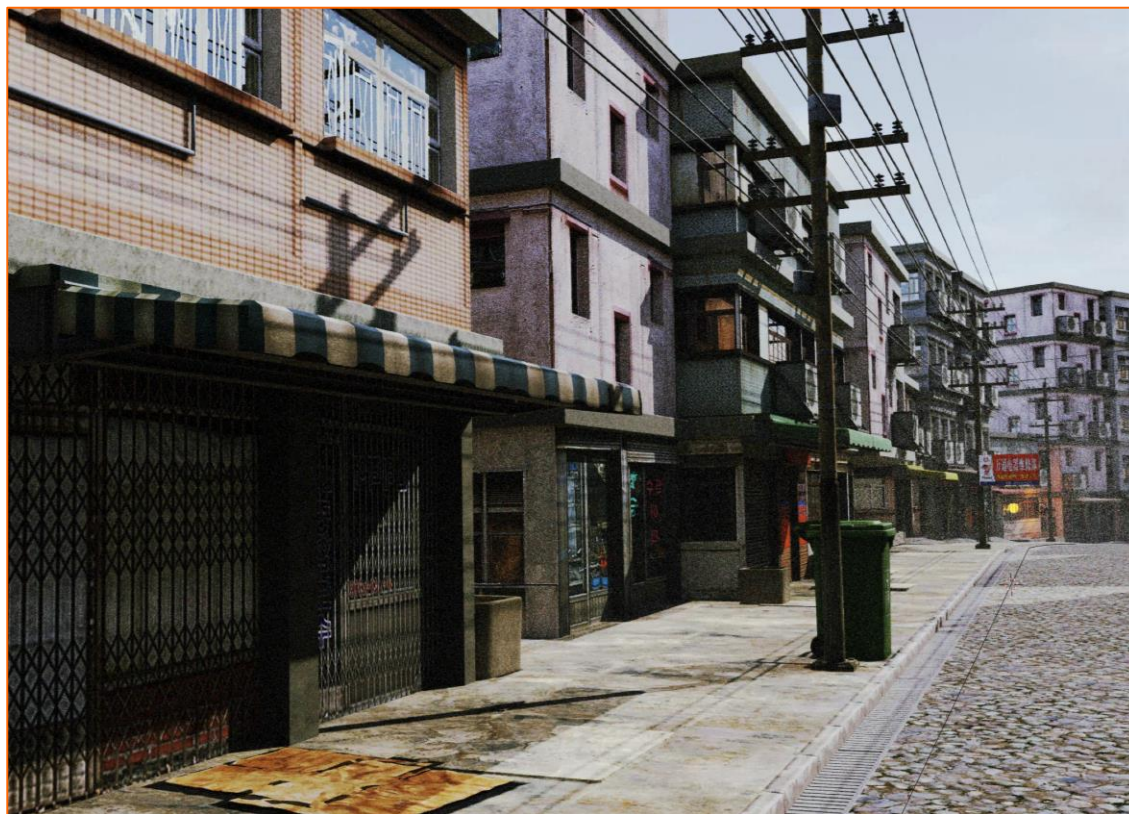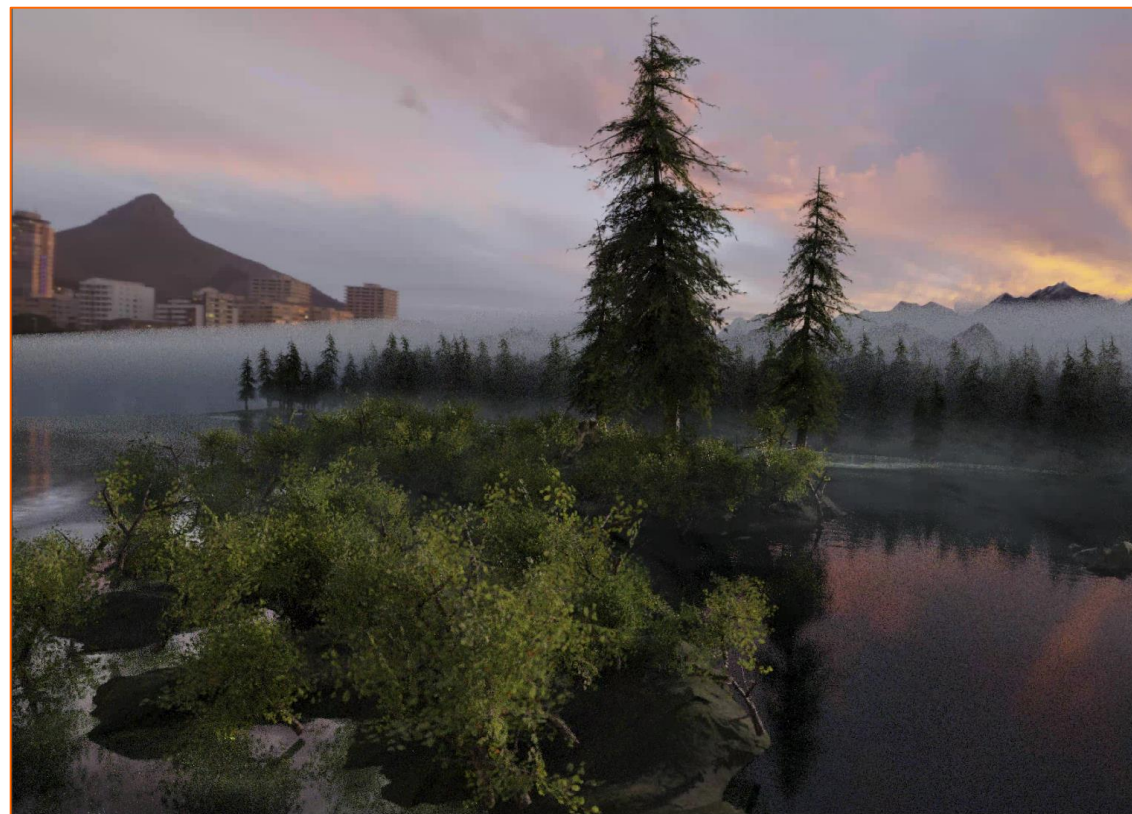

**WireFrame  
Mode**

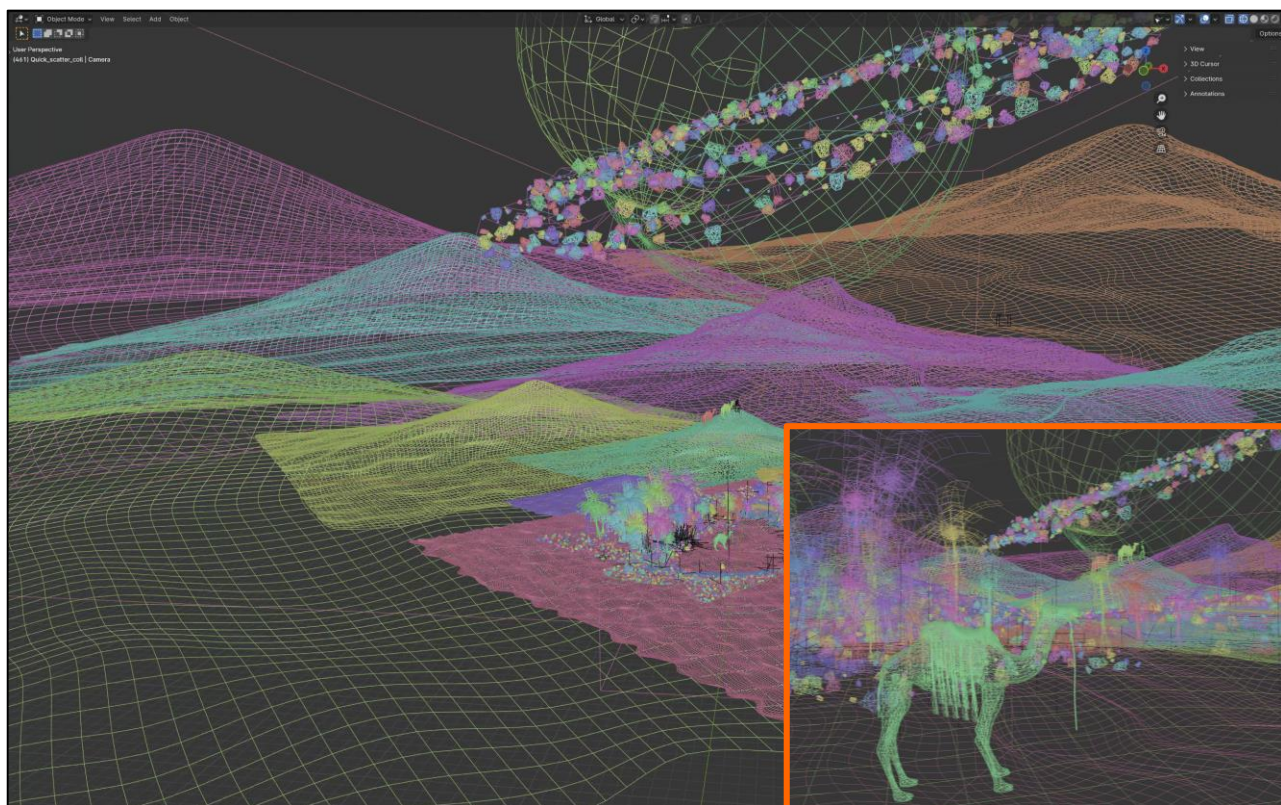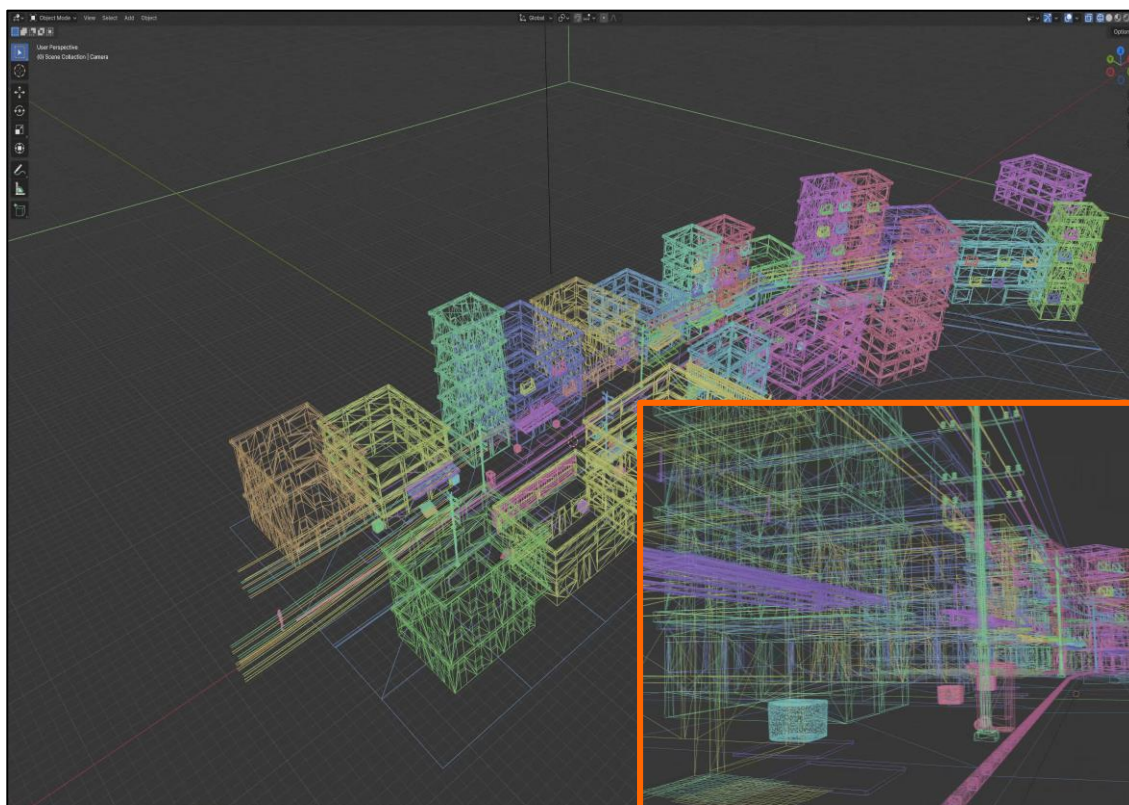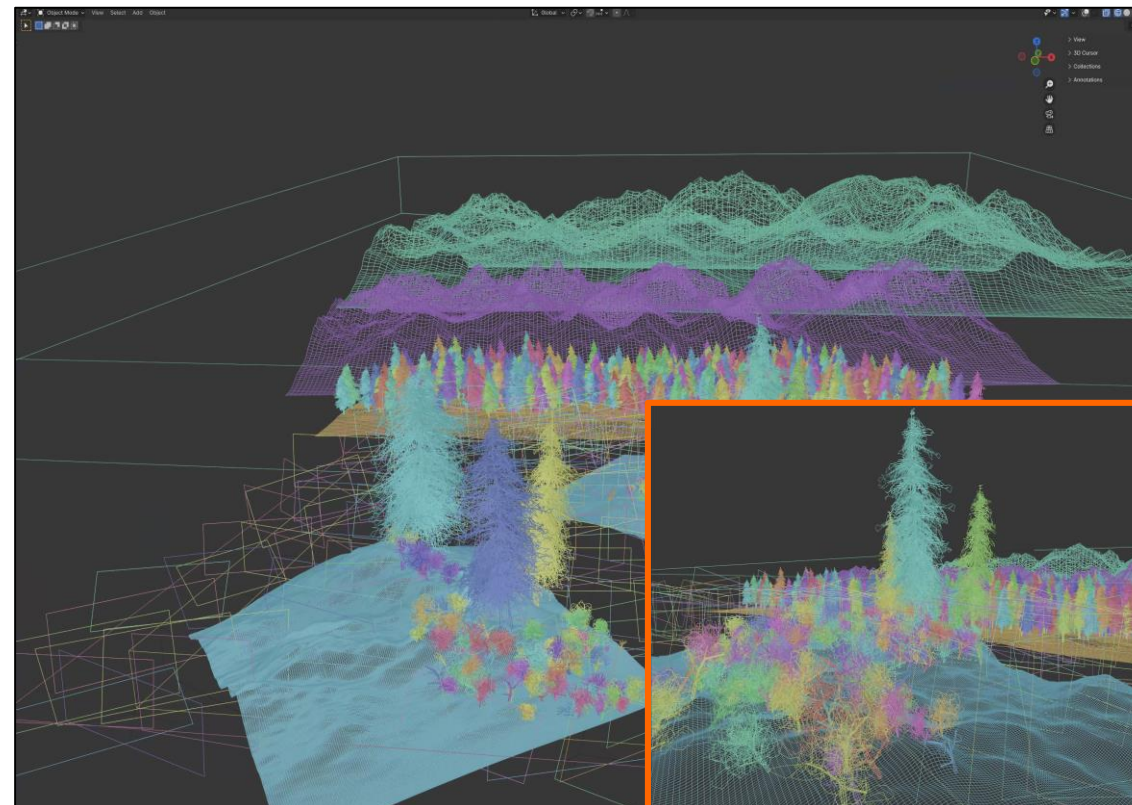

**Desert**

**City Blocks**

**Lake**



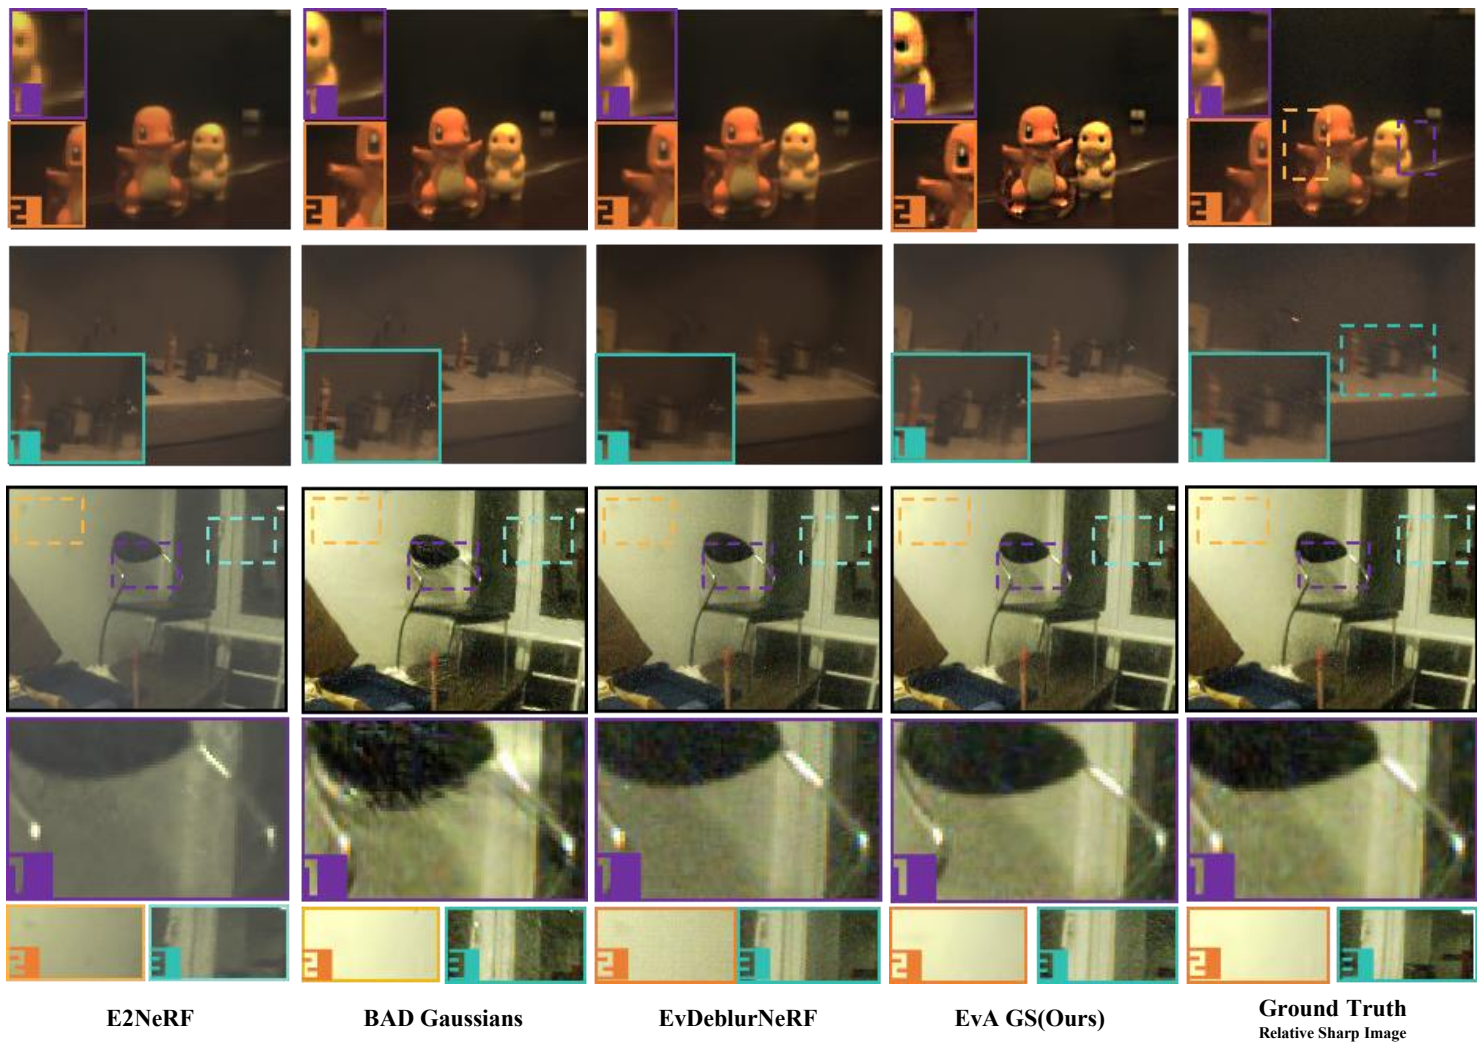

Supplement: Supplementary file 1 [file appendix_outdoors.pdf]
